# Supplementary material for: Finite Sample Frequency Domain Identification
Source: arXiv:2404.01100 source file (2024-09-05)
Supplement: Supplementary file 1 [file appendix_missing_proofs.tex]

\subsection{Proof of Lemma~\ref{lem:PE}}
Fix an experiment index $i$. Since $u^{(i)}_t$ is periodic with period $M$ and $\Np$ is an integer, we have
\begin{equation*}
\begin{aligned}
   \sum_{t=0}^{N-1}u^{(i)}_te^{-j\omega_k t}&=\sum_{\tau=0}^{\Np-1}\sum_{t=0}^{M-1}u^{(i)}_te^{-j\omega_k (M\tau+t)}\\
   &=\paren{\sum_{\tau=0}^{\Np-1}e^{-j\frac{2\pi k}{\Np}\tau}}\paren{\sum_{t=0}^{M-1}u^{(i)}_te^{-j\omega_k t}}
\end{aligned}
\end{equation*}
Therefore, we obtain
\begin{equation*}
\begin{aligned}
   U^{(i)}_{\Np\ell}&=\sqrt{\Np}\tilde{U}^{(i)}_l,\,\text{for }\Np\ell, \ell\in[M]\\
   U^{(i)}_k&=0,\,\text{elsewhere. }
\end{aligned}
\end{equation*}
For $k=\Np\ell$ we have
\[
U_kU^*_k=\Np \tilde{U}_\ell\tilde{U}^*_\ell\succeq N_p \sigma^2_{u,\ell}I_{\du}.\tag*{\qed}
\]

\subsection{Proof of Theorem~\ref{thm:finite_sample_ETFE}}
By~\eqref{eq:estimation_error}, the estimation error is upper bounded by
\[
\opnorm{\hat{G}_k-G(e^{j\omega_k})}\le \opnorm{V_k}\opnorm{U_k^{-1}}+\opnorm{T_{k,N}}\opnorm{U^{-1}_k}.
\]
Invoking Lemma~\ref{lem:noise_concentration}, we have with probability at least $1-\tilde{\delta}$
\begin{align*}
\opnorm{V_k}&\le \sqrt{\tr(\Phi_{v,N}(k))}+2\tilde{s}\sqrt{\tr(\Phi_{v,N}(k))}\\
\tilde{s}^2\tr(\Phi_{v,N}(k))&=c'\frac{K^4}{\sigmae^4}\opnorm{\Phi_{v,N}(k))}(\log(1/\tilde{\delta})+\du),
\end{align*}
for some universal constant $c'$. Set $\delta/M=\tilde{\delta}$ and consider a union bound over all $\ell\in[M]$. Then, with probability at least $1-\delta$, for all $k=\Np\ell$, $\ell\in[M]$ 
\begin{multline}
\opnorm{V_k}\le \sqrt{\dy}\sqrt{\opnorm{\Phi_{v,N}(k)}}\\+\sqrt{c'}\frac{K^2}{\sigmae^2}\sqrt{\opnorm{\Phi_{v,N}(k))}}\sqrt{\log(M/\delta)+\du},
\end{multline}
where we used $\tr(\Phi_{v,N}(k))\le \dy\opnorm{\Phi_{v,N}(k)}$.
The proof now follows from Lemma~\ref{lem:deterministic_transient} and Lemma~\ref{lem:PE}.\hfill$\qed$
\subsection{Proof of Theorem~\ref{thm:sup_norm_guarantees}}
It follows directly from Theorem~\ref{thm:finite_sample_ETFE} and
\[
\opnorm{G(e^{j\omega})-\hat{G}^N(e^{j\omega})}\le \frac{\pi}{M}\snorm{G}_{\star}+\opnorm{G(e^{j\omega_{\ell N_p}})-\hat{G}_{\ell N_p}}.\tag*{\qed}
\]
